# Supplementary material for: Conditional Generative Denoiser for Nighttime UAV Tracking
Source: arXiv:2409.16834 source file (2024-09-25)
Supplement: Supplementary file 1 [file supplementay_proof_of_CGDenoiser.pdf]

# Supplementary proof of CGDenoiser

By Yucheng Wang

July 2024

## 1 Nomenclature

| Notation | Description |
| --- | --- |
| $c$ | Ground truth of clean image |
| $x$ | Noise map |
| $z_x$ | Latent variable of noise map |
| $k$ | Kernels for conditional refinement |
| $z_k$ | Latent variable of refinement kernels |
| $n_x$ | Noisy image |
| $d_x$ | Preliminarily denoised image |
| $D_x$ | Denoised image |
| $\mathcal{I}(\cdot)$ | Integration of convolution maps |
| $m_k$ | Number of refinement kernels |
| $s_k$ | Size of refinement kernels |

Table 1: Nomenclature

## 2 Proof

To maximize the conditional likelihood: $\log p(D_x \mid n_x)$

$$\propto \log \int_{c,z_x,z_k,x,k} \cdots \int p\left(z_x \mid c\right) p\left(z_k \mid c\right) p\left(x \mid z_x, n_x\right) p\left(k \mid z_k, n_x\right) p(D_x \mid x, k, n_x)$$

$$\overset{k \perp c \mid z_k}{\underset{x \perp c \mid z_x}{=\!=\!=}} \log \int_{c,z_x,z_k,x,k} \cdots \int p\left(x, z_x \mid c, n_x\right) p\left(k, z_k \mid c, n_x\right) p(D_x \mid x, k, n_x)$$

$$= \log \int_{c,z_x,z_k,x,k} \cdots \int \frac{p(x,z_x|c,n_x)q(z_x|c)}{q(z_x|c)} \frac{p(k,z_k|c,n_x)q(z_k|c)}{q(z_k|c)} p(D_x \mid x, k, n_x)$$

$$= \log \mathbb{E}_{q(z_x,z_k|c)}[\frac{p(x,z_x|c,n_x)}{q(z_x|c)} \frac{p(k,z_k|c,n_x)}{q(z_k|c)} p(D_x \mid x, k, n_x)]$$

with the concavity of logarithm and according to Jensen's inequality:

$$\geq \mathbb{E}_{q(z_x|c)}[\log \frac{p(x,z_x|c,n_x)}{q(z_x|c)}] + \mathbb{E}_{q(z_k|c)}[\log \frac{p(k,z_k|c,n_x)}{q(z_k|c)}] + \mathbb{E}_{q(z_x,z_k|c)}[\log p(D_x \mid x, k, n_x)]$$

$$= \mathbb{E}_{q(z_x|c)}[\log \frac{p(x|z_x,c,n_x)p(z_x|c,n_x)}{q(z_x|c)}] + \mathbb{E}_{q(z_k|c)}[\log \frac{p(k|z_k,c,n_x)p(z_k|c,n_x)}{q(z_k|c)}]$$

$$+\mathbb{E}_{q(z_x,z_k|c)}[\log p(D_x \mid x, k, n_x)]$$

$$= \mathbb{E}_{q(z_x|c)}[\log p\left(x \mid z_x, c, n_x\right)] - \mathrm{KL}[q(z_x \mid c) \| p(z_x \mid c, n_x)] + \mathbb{E}_{q(z_k|c)}[\log p\left(k \mid z_k, c, n_x\right)]$$

$$-\mathrm{KL}[q(z_k \mid c) \| p(z_k \mid c, n_x)] + \mathbb{E}_{q(z_x,z_k|c)}[\log p(D_x \mid x, k, n_x)]$$

$$= \mathbb{E}_{q(z_x,z_k|c)}[\log p\left(x \mid z_x, c, n_x\right) p\left(k \mid z_k, c, n_x\right) p(D_x \mid x, k, n_x)] - \mathrm{KL}[q(z_x \mid c) \| p(z_x \mid c, n_x)]$$

$$-\mathrm{KL}[q(z_k \mid c) \| p(z_k \mid c, n_x)]$$

$$\overset{k \perp c \mid z_k}{\underset{x \perp c \mid z_x}{=\!=\!=}} \mathbb{E}_{q(z_x,z_k|c)}[\log p\left(x \mid z_x, n_x\right) p\left(k \mid z_k, n_x\right) p(D_x \mid x, k, n_x)] - \mathrm{KL}[q(z_x \mid c) \| p(z_x \mid c, n_x)]$$

$$-\mathrm{KL}[q(z_k \mid c) \| p(z_k \mid c, n_x)]$$

$$\propto \mathbb{E}_{q(z_x,z_k|c)}[p\left(x \mid z_x, n_x\right) p\left(k \mid z_k, n_x\right) p(D_x \mid x, k, n_x)] - \mathrm{KL}[q(z_x \mid c) \| p(z_x \mid c, n_x)]$$

$$-\mathrm{KL}[q(z_k \mid c) \| p(z_k \mid c, n_x)]$$

$$= \mathbb{E}_{q(z_x,z_k|c)p(x|z_x,n_x)p(k|z_k,n_x)}[p(D_x \mid x, k, n_x)] - \mathrm{KL}[q(z_x \mid c) \| p(z_x \mid c, n_x)]$$

$$-\mathrm{KL}[q(z_k \mid c) \| p(z_k \mid c, n_x)]$$

The loss function of CGDenoiser with trainable parameters:

$$\mathcal{L}_{CGD}(\theta_x, \theta_k, \phi_x, \phi_k, \epsilon) =$$

$$-\mathbb{E}_{q_\theta(z_x, z_k|c) p_{\phi_x}(x|z_x, n_x) p_{\phi_k}(k|z_k, n_x)}[p_\epsilon(D_x \mid x, k, n_x)] + \mathrm{KL}[q(z_x \mid c) \| p_{\phi_x}(z_x \mid c, n_x)]$$

$$+\mathrm{KL}[q(z_k \mid c) \| p_{\phi_k}(z_k \mid c, n_x)].$$

where the prior $q(z_x \mid c) \sim \mathcal{N}(\mathbf{0}, \mathbf{I})$, $q(z_k \mid c) \sim \mathcal{N}(\mathbf{0}, \mathbf{I})$. Assuming the clean image contains sufficient prior knowledge for the posterior approximation network and $z_x, z_k$ follow multi-dimensional gaussian distributions $p_{\phi_x}(z_x \mid c, n_x) \sim \mathcal{N}(\mu_{\phi_x}(c), \Sigma_{\phi_x}(c))$, $p_{\phi_k}(z_k \mid c, n_x) \sim \mathcal{N}(\mu_{\phi_k}(c), \Sigma_{\phi_k}(c))$, the objective denoised image $p_\epsilon(D_x \mid x, k, n_x) \sim \mathcal{N}(c, \sigma)$, then with $d_x = n_x - x$, $D_x \triangleq \mathcal{I}(d_x * k_1, d_x * k_2, ..., \ d_x * k_{m_k})$ one can obtains:

$$\theta_x^*, \theta_k^*, \phi_x^*, \phi_k^*, \epsilon^* =$$

$$\arg \min_{\theta_x, \theta_k, \phi_x, \phi_k, \epsilon} \mathbb{E}_{q_\theta(z_x, z_k|c) p_{\phi_x}(x|z_x, n_x) p_{\phi_k}(k|z_k, n_x)} \left[ \frac{(\|c - \mathcal{I}_\epsilon(x, k, n_x)\|)^2}{2\sigma} \right] + D_{\mathrm{KL}[z_x]} + D_{\mathrm{KL}[z_k]}$$

The first term can be quantified and optimized by Monte Carlo simulation and pixel-wise loss. The latter two terms can be explicitly expressed and narrowed as in classical variational autoencoder. Also it is worth noting that $\sigma$ serves to balance the regularization and the construction loss.

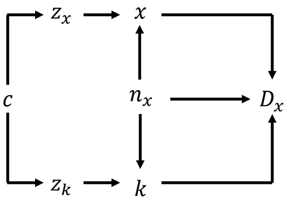


Figure 1: Directed acyclic graph (DAG) of CGDenoiser
